# Supplementary material for: MIMIC: Masked Image Modeling with Image Correspondences
Source: arXiv:2306.15128 source file (2024-05-16)
Supplement: Supplementary file 1 [file 10_appendix_reconstruction_experiment.tex]

\section{Details on the reconstructions experiment}
In this study, we collected 500 test image pairs from the Gibson dataset to ensure a fair evaluation process. We made a careful selection to exclude scenes present in the \datasetlarge dataset, and confirmed that the \baseline dataset did not include Gibson scenes.
 Following this, we employed a random masking approach on the target image, utilizing the same masking matrix for inputs of both the model trained on MIMIC3M and the one trained on MV-Habitat. The purpose of this consistent masking procedure was to enable a comparative assessment of the reconstruction performance on equivalent image patches.
 Then, each model separately reconstructed the masked target view using the reference view. For the overall reconstruction loss, we got the average over 500 test pairs, which reconstruction loss for each pair was an average of l2 loss over masked pixels. See reconstruction examples of both models in Figure \ref{fig:recons}.

\begin{figure}[ht]
    \centering
    \includegraphics[width=\textwidth]{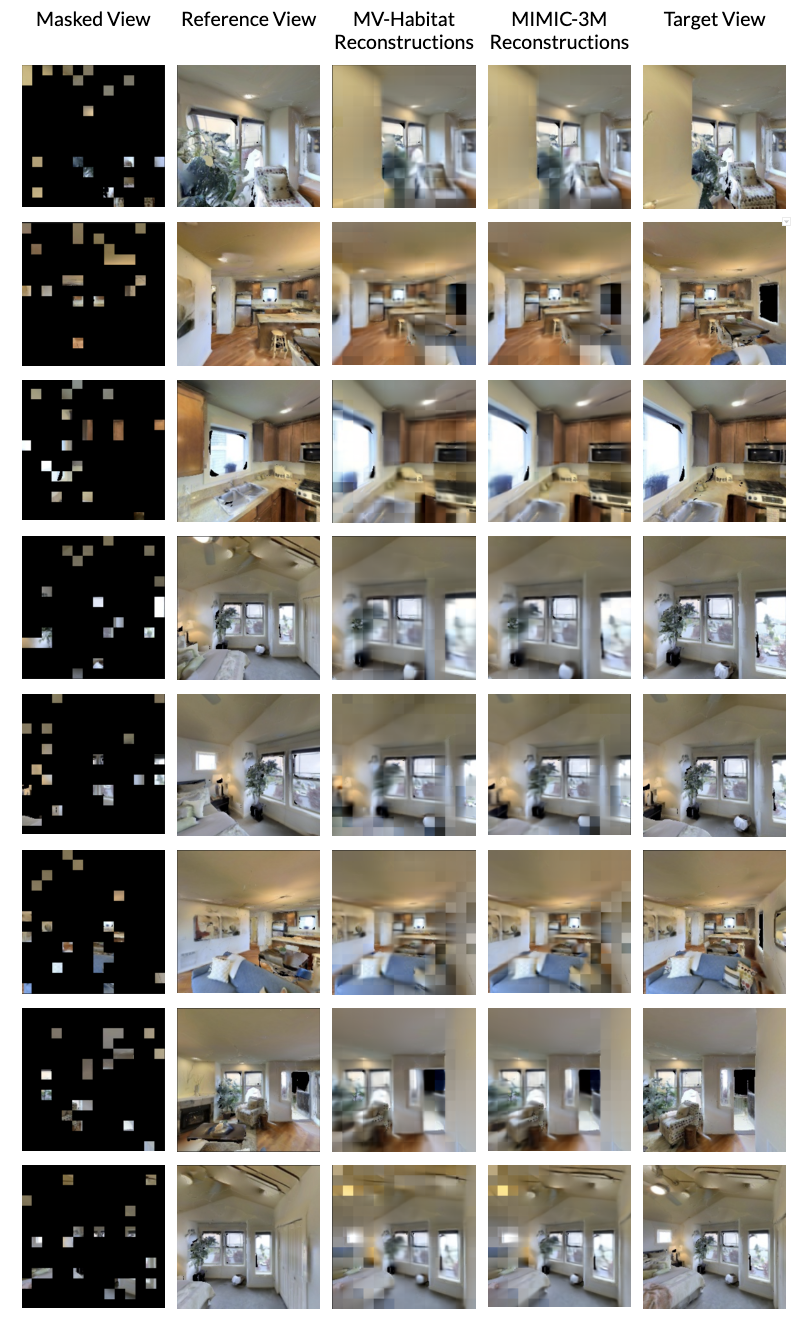}
    \caption{Visualizations of the reconstructions}
    \label{fig:recons}
\end{figure}
